# Supplementary material for: Biocompatible Vaterite Carriers Enable Multimodal Quantum Sensing with Nanodiamonds
Source: arXiv:2608.09434 source file (2026-08-17)
Supplement: Supplementary file 1 [file Appendices.tex]

%\section {\Large\textbf{Appendix A: Cathodoluminescence Characterization of Vaterite}}

Figure~\ref{fig:A1} shows the cathodoluminescence (CL) spectrum of vaterite particles collected under 30~keV electron-beam excitation. The spectrum exhibits a prominent emission peak at approximately 405~nm, corresponding to the intrinsic luminescence of the vaterite crystal lattice. This measurement supports the statement in the main text, confirming that the observed peak originates from the vaterite host itself.
\begin{figure}[h]
\centering
\includegraphics[width=0.5\textwidth]{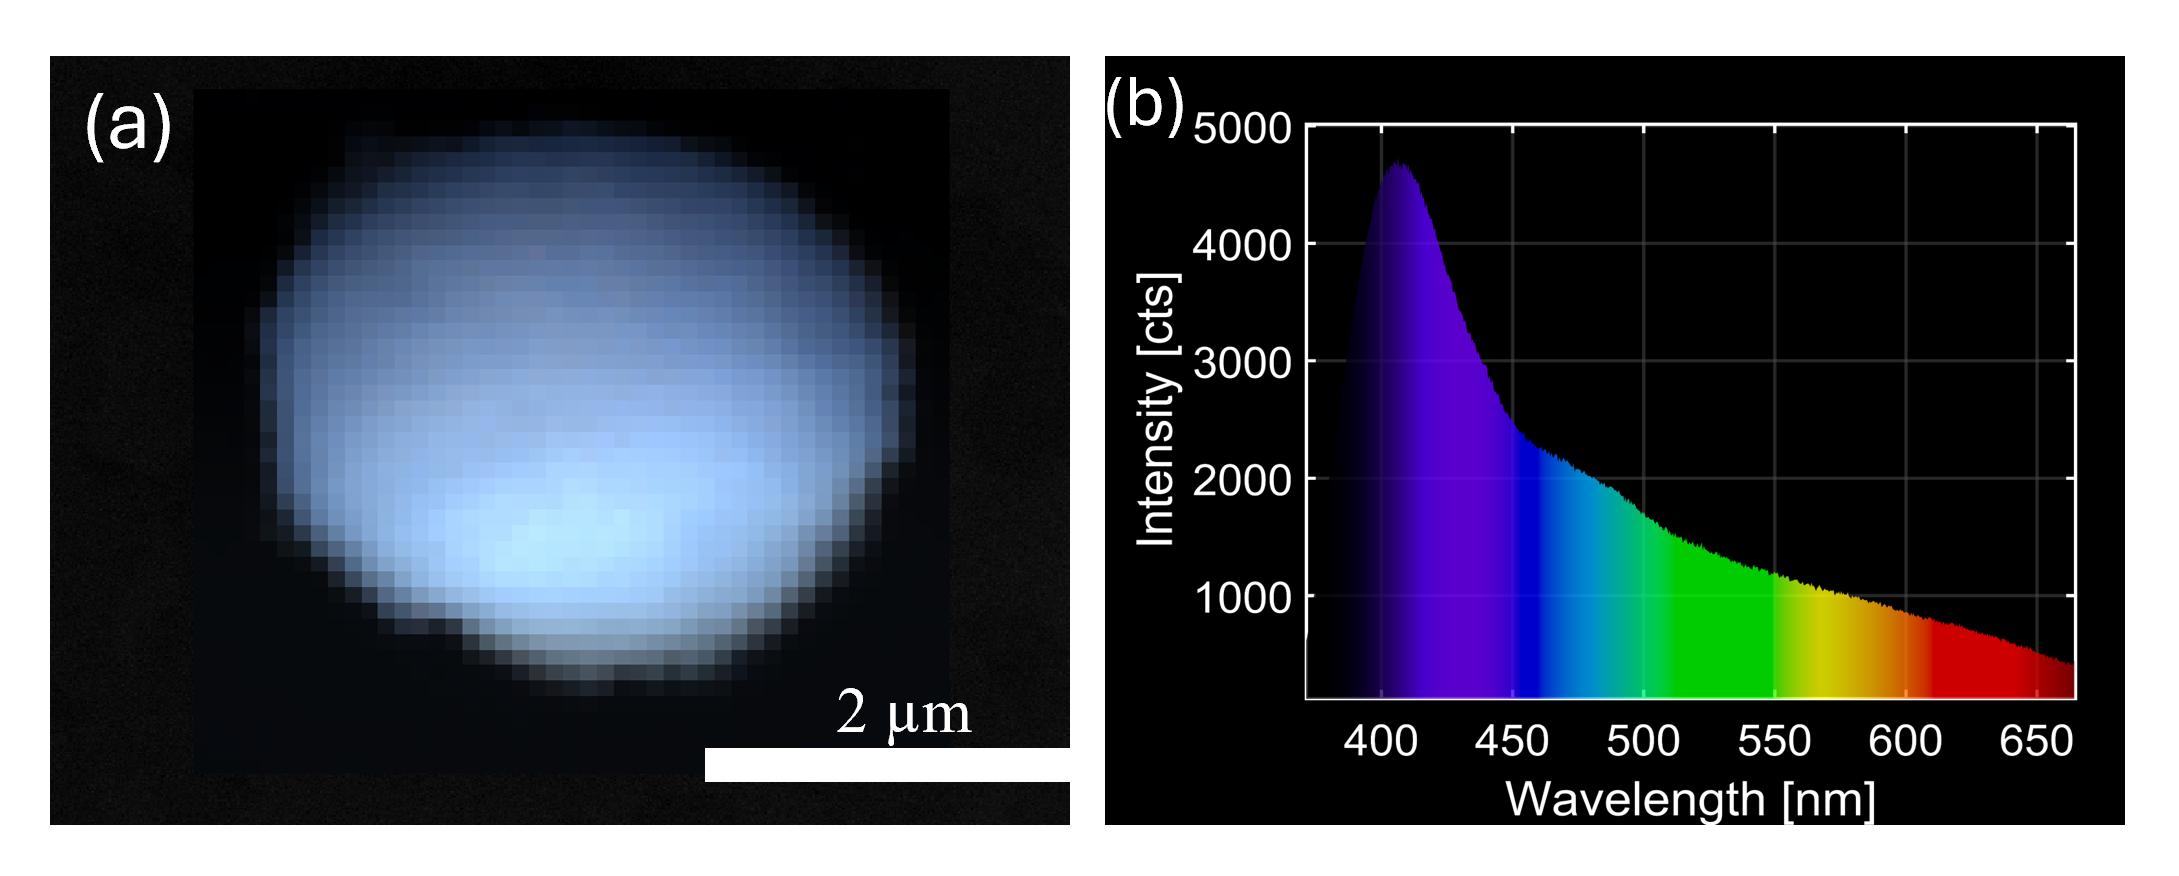}
\caption{Cathodoluminescence characterization of vaterite. (a) CL maps were acquired using a 30~keV electron beam at 17~nA. (b) CL spectrum of vaterite, showing a prominent peak at 405~nm corresponding to the intrinsic luminescence of the vaterite host.}
    \label{fig:A1}
\end{figure}
